# Supplementary material for: Investigations of fundamental symmetries with the electron-positron systems
Source: arXiv:1805.06009 source file (2018-05-15)
Supplement: Supplementary file 1 [file AppendixC.tex]

\chapter{Kinematic fit with constrained least squares minimization}\label{appendix:kinfit}

%\begin{equation}
%   \label{eq:fit_system}
%   \begin{bmatrix}
%     \mathbf{V}^{-1} &  \mathbf{D}^T \\
%     \mathbf{D} & 0
%   \end{bmatrix}
%   \begin{bmatrix}
%     \mathbf{\Delta x} \\
%     \mathbf{\lambda}
%   \end{bmatrix}
  
% \end{equation}
